# Supplementary material for: A favorably-scaling natural-orbital functional theory based on higher-order occupation probabilities
Source: arXiv:1309.3929 ancillary file (2015-06-20)
Supplement: Supplementary file 1 [file SI.pdf]

# Supporting Information:

A favorably scaling natural-orbital functional theory based on higher-order occupation probabilities

by R. Gebauer, M. H. Cohen, and R. Car

## S1. POSITIVE MATRIX ELEMENTS

The proof of the sign conjecture for positive matrix elements utilizes NSO-based Brillouin-Wigner perturbation theory (BWPT). An SD basis is constructed from the NSOs of the true ground-state wave function $\Psi_G$ of $\hat{H}$, which has parts diagonal, $\hat{H}^d$, and off-diagonal, $\hat{U}^{od}$, in the basis. $\hat{U}^{od}$ is the off-diagonal part of the $N$-electron Coulomb interaction. The eigenfunctions of $\hat{H}^d$ are the SD $\Phi_{\mathbf{k}}$, and $E_{\mathbf{k}}$ are the corresponding eigenvalues. $E_{\mathbf{0}} = \inf\{E_{\mathbf{k}}\}$ is the lowest of those and $\Phi_{\mathbf{0}}$ the associated eigenfunction. $\hat{U}^{od}$ is treated as a perturbation on $\hat{H}^d$; it generates $\Psi_G$ from $\Phi_{\mathbf{0}}$. The expansion coefficients $C_{\mathbf{k}}$ of $\Psi_G$ in the $\Phi_{\mathbf{k}}$ are

$$C_{\mathbf{k}} = C_{\mathbf{0}}\,\delta_{\mathbf{k},\mathbf{0}} + (1-\delta_{\mathbf{k},\mathbf{0}}) \sum_{\mathbf{l}\neq\mathbf{k}} \left[E_G - E_{\mathbf{l}}\right]^{-1} \left(\hat{U}^{od}\right)_{\mathbf{kl}} C_{\mathbf{l}}. \tag{S1}$$

The $a^{th}$-order term in the expansion of $C_{\mathbf{k}}$, $\mathbf{k}\neq\mathbf{0}$, is obtained by iterating Eq. **S1**:

$$C^{(a)}_{\mathbf{k}} = \sum_{\mathbf{l}_1\cdots\mathbf{l}_{a-1}} \left[E_G - E_{\mathbf{l}_{a-1}}\right]^{-1} \left(\hat{U}^{od}\right)_{\mathbf{k}\mathbf{l}_{a-1}} \cdots \cdots \left[E_G - E_{\mathbf{l}_1}\right]^{-1} \left(\hat{U}^{od}\right)_{\mathbf{l}_1\mathbf{0}} C_{\mathbf{0}}. \tag{S2}$$

Setting the sign of $C_{\mathbf{k}}$ equal to that of the lowest order term in its BWPT expansion, the $a(\mathbf{k})^{th}$ term, is variational. An excited NSO is one present in $\Phi_{\mathbf{k}}$ and not in $\Phi_{\mathbf{0}}$. Classify $C_{\mathbf{k}}$ by the number of its occupied excited NSOs and assign values $l \leq N$ to the index $l$ if $\psi_l$ is present in $\Phi_{\mathbf{0}}$ and $l > N$ if excited from $\Phi_{\mathbf{0}}$. Give $r_l$ the value 0 when $l \leq N$ and 1 when $l > N$. $R(\mathbf{k}) = \sum_{l\in\mathbf{k}} r_l$ is the number of excited NSOs in $\Phi_{\mathbf{k}}$ obtained by counting the number of indices $> N$ in $\mathbf{k}$. The PDC restricts $R(\mathbf{k})$ to be either odd or even for all $\mathbf{k}$. If $C_{\mathbf{0}}$ is finite, $R(\mathbf{k})$ must be even, $\forall\mathbf{k}$, as $R(\mathbf{0}) = 0$. In the lowest order $a(\mathbf{k})$ of $C_{\mathbf{k}}$, each matrix element on its right hand side of Eq. **S2** increases the values of 2 distinct $r_k$ from 0 to 1. Consequently

$$a(\mathbf{k}) = \frac{1}{2}R(\mathbf{k}),$$

each of the $a(\mathbf{k})$ matrix elements having changed 2 indices from $\leq N$ to $> N$. As each matrix element in Eq. **S2** is positive and denominator negative because $E_G < E_{\mathbf{k}}, \quad \forall \mathbf{k} \neq \mathbf{0}$, we obtain

$$\operatorname{sgn}\{C_{\mathbf{k}}\} = (-1)^{a(\mathbf{k})} = (-1)^{\frac{1}{2}R(\mathbf{k})} \tag{S3}$$

as our variational approximation. Eq. **S3** implies

$$s(ii'\mathbf{k}) = (-1)^{\frac{1}{2}R(ii'\mathbf{k})}. \tag{S4}$$

$R(ii'\mathbf{k})$ can be decomposed into contributions from $ii'$ and from $\mathbf{k}$:

$$R(ii'\mathbf{k}) = R(ii') + R(\mathbf{k}). \tag{S5}$$

$R(ii'\mathbf{k})$ is even. Eqs. **S4** and **S5** imply that

$$s(ii'\mathbf{k}) = (-1)^{\frac{1}{2}[R(ii')+R(\mathbf{k})]}.$$

The product of two signs in **11** becomes

$$s(ii'\mathbf{k})s(jj'\mathbf{k}) = (-1)^{\frac{1}{2}[R(ii')+R(jj')]}(-1)^{R(\mathbf{k})}. \tag{S6}$$

$R(ii')$ and $R(\mathbf{k})$ must both be even or both odd. If $R(ii')$ is even, so must be $R(\mathbf{k})$ and therefore $R(jj')$. If $R(ii')$ is odd, so must be $R(\mathbf{k})$ and therefore $R(jj')$. With this added information, Eq. **S6** implies that

$$s(ii'\mathbf{k})s(jj'\mathbf{k}) = (-1)^{\frac{1}{2}[R(ii')+R(jj')]}(-1)^{\mathbb{P}(ii'\text{or } jj')}, \tag{S7}$$

with

$$\mathbb{P}(ii'\text{or } jj') = \begin{cases} 0 & ii', jj'\text{even} \\ 1 & ii', jj'\text{odd} \end{cases}$$

$\mathbb{P}(ii'\text{or } jj')$ can be partitioned into $\frac{1}{2}\mathbb{P}(ii') + \frac{1}{2}\mathbb{P}(jj')$. Inserting this into Eq. **S7** proves the conjecture **12** with

$$s(ii') = (-1)^{\frac{1}{2}[R(ii')+\mathbb{P}(ii')]} \tag{S8}$$

$$s(jj') = (-1)^{\frac{1}{2}[R(jj')+\mathbb{P}(jj')]}, \tag{S9}$$

$R(ii')$ or $R(jj')$ can take only 3 values: 0, 1, and 2. The resulting signs are

| $R(ii')$ | $\mathbb{P}(ii')$ | $s(ii')$ |
|---|---|---|
| 0 | 0 | $+$ |
| 1 | 1 | $-$ |
| 2 | 0 | $-$ |

*Table S1. Sign rule for positive matrix elements*

As derived, Eqs. **S8**–**S9** and table S1 apply to the signs of the coefficients in the expansion of the ground state $\Psi_G$ in SD comprised of the NSO of $\Psi_G$. Our goal is to find a sign rule for the coefficients in the expansion **1** of the trial function $\Psi$. We do so by making an arbitrary association of each NSO with index $i$ of $\Psi$ with an NSO of the same index $i$ of $\Psi_G$. If the NSO $i$ is considered occupied in $\Psi_G$, its associated NSO is considered "occupied" in $\Psi$ as well, and similarly for unoccupied NSOs. We now make the variational approximation that the signs $s(ii'\mathbf{k})$ of each $C(ii'\mathbf{k})$ in the expansion **1** of the trial function $\Psi$, are identical to the signs of the lowest-order terms of the corresponding coefficients $C(ii'\mathbf{k})$ in the expansion of the true ground state $\Psi_G$. It follows that Eqs. **S8** and **S9** and the table then apply as well to the signs of the coefficients in the expansion of the trial function. Eqs. **S8**–**S9** and the table thus constitute our sign rule. It is simple, variational, and of algebraic complexity, scaling as $M^2$. The rule was derived from three assumptions: (1) The PDC was imposed on the SD basis for expanding the ground state. (2) Each ground-state coefficient $C(ii'\mathbf{k})$ was given the sign of the lowest order term in its BWPT series. (3) All matrix elements $K(ii', jj') - K(ii', j'j)$ are positive in the bases generated both by the ground-state and the trial-function NSOs. The rule is exact in the limit of weak correlation under the PDC, and its validity extends beyond that limit. There are 4 pairs of values for $R(ii')$ and $R(jj')$: $(0,0)$; $(0,2)$; $(1,1)$; $(2,2)$. The product $s(ii')s(jj')$ is negative only in the $(0,2)$ case, implying that the excitation of pairs is the primary driver by which correlation lowers the energy below the HF value, an intuitively obvious result.

## S2. MINIMIZATION OF THE ENERGY

The minimization of the energy functional $E$ in **28** of the main text is performed using a damped Car-Parrinello dynamics approach. The NOs $\{\phi_i\}$ are propagated in 'time' $t$ (the relaxation time) according to

$$\frac{d^2}{dt^2}|\phi_i\rangle = |F_i\rangle - \gamma \frac{d}{dt}|\phi_i\rangle + \sum_j \Lambda_{ij} S|\phi_j\rangle, \tag{S10}$$

where $\gamma$ is a damping coefficient, the $\Lambda_{ij}$ are Lagrange multipliers that enforce orthonormality of the NOs, and $S$ is the overlap matrix. The generalized force $|F_i\rangle$ is defined as

$$|F_i\rangle = |g_i\rangle - \frac{1}{2}\sum_j \left(\langle\phi_j|g_i\rangle + \langle\phi_i|g_j\rangle\right) S|\phi_j\rangle.$$

The vectors $|g_i\rangle$ are given by $|g_i\rangle = -\frac{\partial E}{\partial \langle \phi_i|}$. This definition of $|F_i\rangle$ ensures that the forces lead to a quasi-unitary rotation within the space of the NO's. The small loss of orthogonality accumulated in one time step is corrected by the Lagrange multipliers.

The occupation probabilities $p_1$ and $p_{11}$ are written as

$$p_1(i) = \frac{1}{2}\left(\text{erf}(x(i)) + 1\right) \qquad p_{11}(ij) = \text{SUP} + \left(p_1(<) - \text{SUP}\right)\left(\text{erf}(X(ij)) + 1\right),$$

where SUP is defined as $\sup\left(p_1(i) + p_1(j) - 1, 0\right)$. The parameters $x(i)$ and $X(ij)$ vary from $-\infty$ to $+\infty$. This functional form automatically satisfies the bounds for $p_{11}$ and for $p_1$ given, respectively, in **8** and below **5** of the main text.

The $x(i)$ and $X(ij)$ are optimized simultaneously with the NO's by damped dynamics equations similar to Eq. **S10**, in which Lagrange multipliers enforce the sum rules for the $p_1$ and the $p_{11}$. The condition **9** of the main text is imposed by adding a penalty function to the energy functional.

Typically the infimum of the functional is reached after a few thousand steps. No effort was made to optimize this protocol.

## S3. DISSOCIATION CURVES FOR DIMERS $H_2$, LIH, AND HF

In the following, we show the dissociation curves for three dimers, obtained at various levels of theory. Notice that for $H_2$ we used the larger cc-pVTZ basis set.

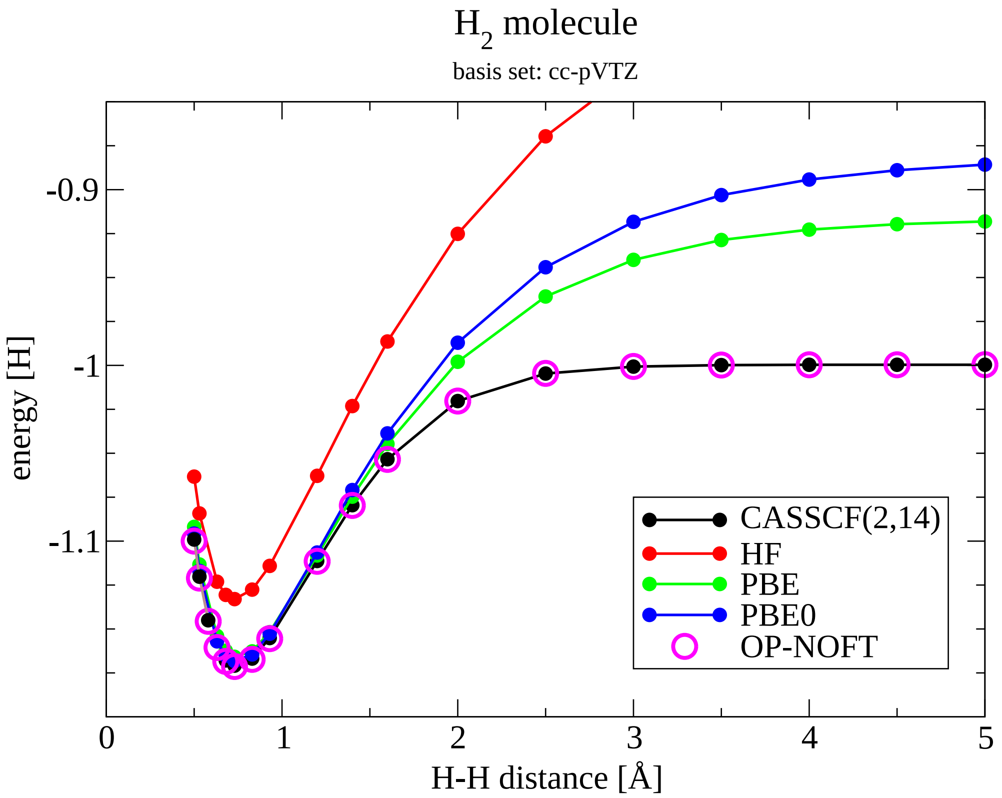


*FIG. S1. Dissociation curve of $H_2$.*

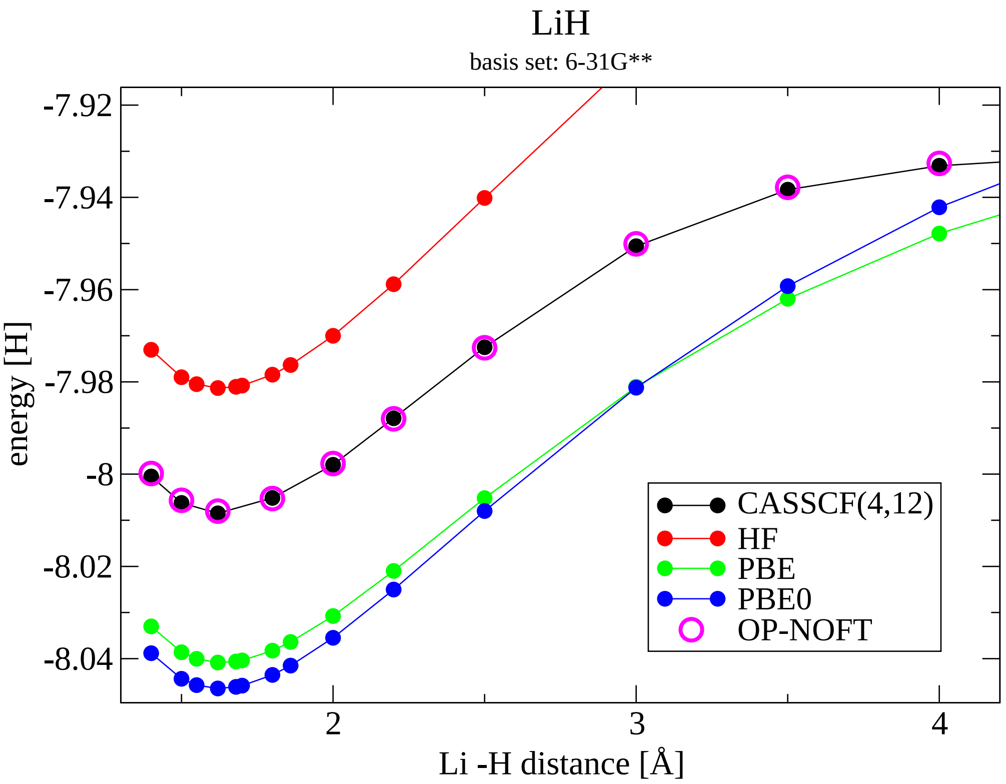


*FIG. S2. Dissociation curve of LiH.*

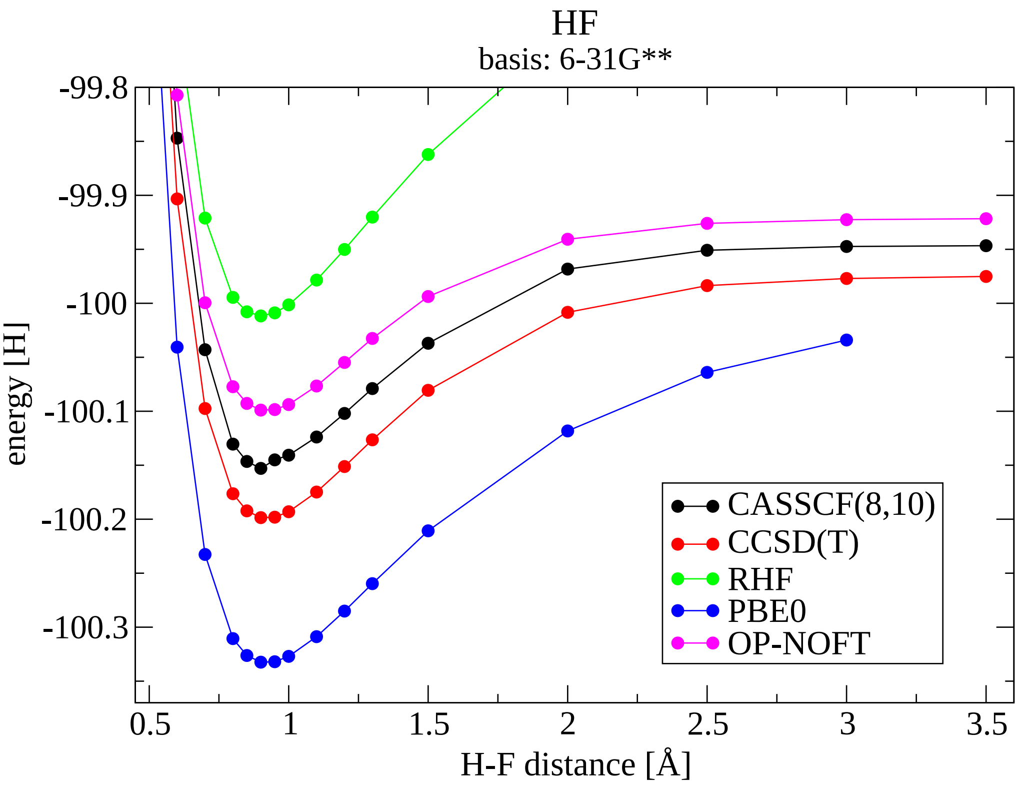


*FIG. S3. Dissociation curve of HF.*

## S4. CONDITIONS FOR TWO-STATE PROBABILITIES IN 4-ELECTRON SYSTEMS

The conditions given in **8–10** of the main text apply to systems with more than four electrons. In the case of four electrons (like, e.g. LiH), each determinant in the $A = 0$ sector is made of two doubly occupied states. In this case, the conditions on the two-state OPs are:

$$\sup(p_1(i) + p_1(j) - 1, 0) \leq p_{11}(ij) \leq p_1(<)$$

$$\sum_{j(\neq i)} p_{11}(ij) = p_1(i),$$

where $p_1(<)$ is the lesser of $p_1(i)$ and $p_1(j)$.

## S5. OCCUPATION NUMBERS AND ENTANGLEMENT ENTROPY

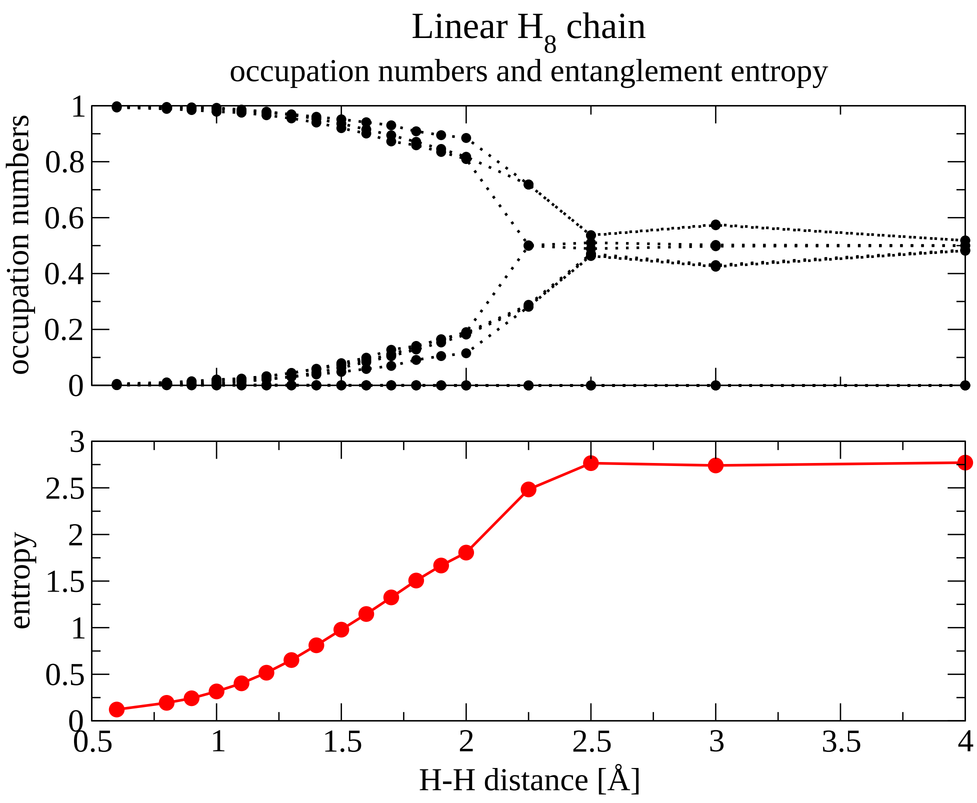


*FIG. S4. Occupation numbers and Von Neumann entanglement entropy in* $H_8$ *as a function of interatomic distance.*

## S6. PAIR-CORRELATION FUNCTION

The parallel spin and anti-parallel spin pair-correlation functions $g_p(\mathbf{r}, \mathbf{r}') = g_{\sigma\sigma}(\mathbf{r}, \mathbf{r}')$ and $g_a(\mathbf{r}, \mathbf{r}') = g_{\sigma\bar{\sigma}}(\mathbf{r}, \mathbf{r}')$ are defined as

$$n_\sigma(\mathbf{r}) n_{\sigma'}(\mathbf{r}') g_{\sigma\sigma'}(\mathbf{r}, \mathbf{r}') = \pi(\mathbf{r}\sigma, \mathbf{r}'\sigma'; \mathbf{r}\sigma, \mathbf{r}'\sigma'), \tag{S11}$$

where $n_\sigma(\mathbf{r}) = \frac{1}{2}\rho(\mathbf{r}, \mathbf{r})$. Plots of the pair correlation functions for the symmetric open-bounded $H_8$ chain are given in Fig. S5. These depict $g$ for electrons of opposite and parallel spins when one electron is placed in the mid-bond (left panel), and in the mid-antibond (right panel) (see discussion in the main text). We notice that the anti-parallel spin correlation shows a positive hump at the location of the tagged electron (dashed vertical line), contrary to what one should expect for a repulsive cusp condition. This is an artifact of the use a

of a finite Gaussian basis, as an infinite set of NO's would be required to exactly reproduce the electron-electron cusp [S1]. For the stretched chain in Fig. S5 (H-H distance = 1.8 Å) the electron-electron cusp has negligible effect on the energy. We find a different behavior near equilibrium (H-H distance = 0.9 Å, plot not shown), where the hump gets replaced by a shallow local minimum of the pair correlation function at coalescence, i.e. a behavior qualitatively in agreement with the strong repulsive interaction between two electrons at short distance. These results are independent of the other approximations made and hold also for $H_4$ where our formula for $\xi$ is exact.

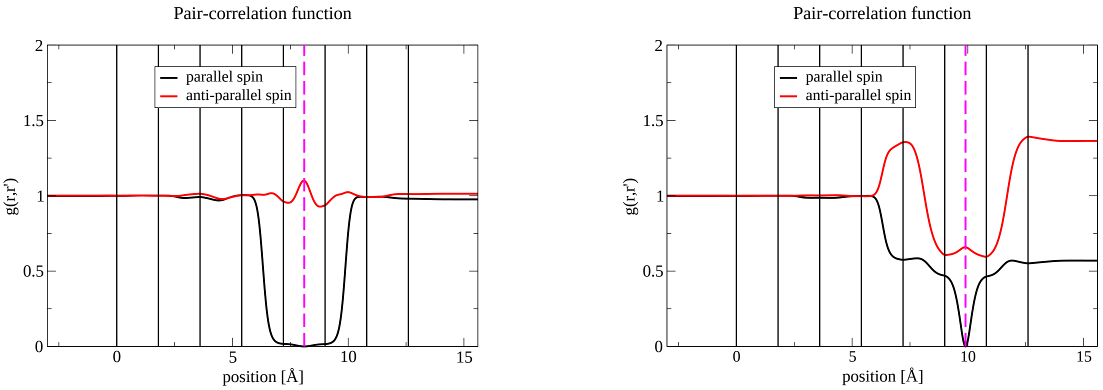


*FIG. S5. Electronic pair-correlation function along the $H_8$ axis when one electron is placed at the position of the vertical dashed line on the molecular axis. The vertical black lines show the atom positions. Left panel: one electron at mid-bond. Right panel: one electron at mid-antibond. The H-H distance is 1.8 Å .*

**References:**

[S1] K. J. H. Giesbertz and R. van Leeuwen, The Journal of chemical physics **139**, 104109 (2013).
